# Supplementary material for: Gradient Informed Proximal Policy Optimization
Source: arXiv:2312.08710 source file (2023-12-14)
Supplement: Supplementary file 1 [file legacy_appendix.tex]

\section{APPENDIX}

\subsection{Proofs}

\vspace{1em}
\subsubsection{Equation~\ref{eq:perturbed-policy}}

To make the function $f$ a bijective function, we should not let its Jacobian matrix $\nabla_{a}f = I + \epsilon \gradQsecond$ to admit null space. That is, its determinant should not be zero. The lower bound of the determinant is 

\begin{align*}
    \det(I + \epsilon \gradQsecond) &\ge \det(I) + \epsilon \det(\gradQsecond) \\
    &= 1 + \epsilon \det(\gradQsecond).
\end{align*}

Therefore, we can guarantee that the determinant is non-zero positive value by making the lower bound positive. We can achieve it by bounding the $\epsilon$ as

\begin{align*}
    |\epsilon| < \frac{1}{\max_{a}|\det(\gradQsecond|)}.
\end{align*}

\vspace{1em}
\subsubsection{Equation~\ref{eq:perturbed-policy-is-not-distribution}}

Here we write $\widetilde{a} = f(a)$ to clarify the relationship between the original action and the perturbed action. Then, following holds:
 
\begin{align*}
    &\qquad \qquad \int_{\widetilde{a}} \tilpieps(\widetilde{a}|s) d\widetilde{a} \\
    &=\int_{a} \pi(a|s) (I + \epsilon \gradQsecond) da \\
    &=\int_{a} \pi(a|s) da + \epsilon \int_{a} \pi(a|s) \gradQsecond da \\
    &=1 + \epsilon \int_{a} \pi(a|s) \gradQsecond da. \\
\end{align*}

\vspace{1em}
\subsubsection{Proposition~\ref{proposition:valid-perturbed-policy}}

\begin{align*}
    &\qquad \qquad \qquad \int_{\bar{a}_{0}}^{{\bar{a}_{1}}} \barpieps(\bar{a}|s) d\bar{a} \\
    &= \int_{a_0}^{a_1} \frac{\pi(a|s)}{1 + \epsilon \det (\gradQsecond)} (I + \epsilon \gradQsecond) da \\
    &\qquad \qquad \quad = \int_{a_0}^{a_1} \pi(a|s) da.
\end{align*}

\subsubsection{Theorem~\ref{theorem:locally-better-policy}}

For a given state $s$, we can estimate the (approximate) expected value of the state under the perturbed policy $\bar{\pi}_{\epsilon}$ as follows. 
\begin{align*}
    &\qquad\quad \int_{\bar{a}} \barpieps(\bar{a}|s)A_{\pi}(s, \bar{a}) d\bar{a} \\
    &= \int_{a} \frac{\pi(a|s)}{1 + \epsilon \det(\gradQsecond)} A_{\pi}(s, a + \epsilon \gradQfirst) (I + \epsilon \gradQsecond) da \\
    &\approx \int_{a} \pi(a|s) \left [ A_{\pi}(s, a) + \epsilon {||\gradQfirst||}^{2} \right ] da \\
    &\qquad (\because \gradQfirst = \nabla_{a}A_{\pi}(s, a)) \\
    &= \int_{a} \pi(a|s)A_{\pi}(s, a) da + \epsilon \int_{a} \pi(a|s) ||\gradQfirst||^2 da.
\end{align*}

Therefore, we can see following holds:

\begin{align*}
    L_{\pi}(\barpieps) &= \int_{s} \rho_{\pi}(s) \int_{\bar{a}} \barpieps(\bar{a}|s)A_{\pi}(s, \bar{a}) d\bar{a} \\
    &= \eta(\pi) + \epsilon \int_{s} \rho_{\pi}(s) \int_{a} \pi(a|s) ||\gradQfirst||^2 da.
\end{align*}

Since $\pi(a|s)$ and $||\gradQfirst||^2$ are positive, $L_{\pi}(\barpieps)$ is greater or equal to $\eta(\pi)$ when $\epsilon > 0$. On the contrary, when $\epsilon < 0$, $L_{\pi}(\barpieps)$ is smaller or equal to $\eta(\pi)$.
